# Supplementary material for: Removal of the Tachyons from the Fermionic Sector of the Quadratic ZX Action for the Exotic Model (E8)
Source: arXiv:2512.08561 ancillary file (2025-12-09)
Supplement: Supplementary file 1 [file E8-MathDec9Final.pdf]

C:\Users\Jadix\Desktop\E8Final\E8-MathDec9Final.nb

THIS MATHEMATICA NOTEBOOK DISCUSSES THE FERMION PROPAGATORS IN THE ZX SECTOR OF THE XM. IT IS EXPLAINED IN MORE DETAIL IN THE PAPER E8, WHICH IS ENTITLED ``Removal of the Tachyons from the Fermionic Sector of the Quadratic ZX Action for the Exotic Model (E8)'' THIS NOTEBOOK TAKES APPROXIMATELY 100 SECONDS TO RUN.

In this notebook we will calculate the propagators for the fermions in the ZX sector. The comments in this notebook will try to explain how the calculations in this notebook work.

We start out with a generic Lagrangian, based on E7, with factors  $k_i$  and masses  $m_i$  and source parameters  $e_i$ . The 16 propagators " $\Delta_n$ " which we write here as "propn", are calculated. They are introduced through the "shifts", which also have some parameters  $M_i$ . The  $M_i$  have no physical meaning--they are included just to keep the dimensions of propn to minus two, in mass terms, and the results we obtain reflect that. This notebook arises from, and uses similar notation to, a notebook which deals with the BRS cohomology in some detail. That notebook will be used for paper E9. The fermionic

Lagrangian here is named “quadfermionlagrangian”, and it consists of a number of pieces labelled with  $k_i$  and  $m_i$  and  $e_i$ . Supersymmetry imposes relations between these parameters, and tachyon removal will impose more relations between them. The story of how these combine is reserved for the papers E9 and E10, now in preparation. In this notebook we are concerned, mostly, with tachyon removal, and the constraints it imposes on the parameters.

Here are the field variables:

In[67]:= **Now**

Out[67]=

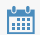

Tue 9 Dec 2025 04:21:11 GMT-7.

In[68]:= **ClearAll["Global`\*"]**

In[69]:= **TimeUsed[ ]**

Out[69]=

0.157

```

In[70]:= amult = {a,  $\psi_0$ ,  $\psi_1$ , f};
abarmult = {abar,  $\psi_{\text{bar}0}$ ,  $\psi_{\text{bar}1}$ , fbar};
umult = {u{0,0}, u{0,1}, u{1,0}, u{1,1},
 $\lambda_0$ ,  $\lambda_1$ ,  $\lambda_{\text{bar}0}$ ,  $\lambda_{\text{bar}1}$ , z, d,  $\eta$ ,  $\omega$ };
xmult = {x{0,0}, x{0,1}, x{1,0},
x{1,1},  $\phi_0$ ,  $\phi_1$ ,  $\chi_0$ ,  $\chi_1$ };
xbarmult = {xbar{0,0}, xbar{0,1}, xbar{1,0},
xbar{1,1},  $\phi_{\text{bar}0}$ ,  $\phi_{\text{bar}1}$ ,  $\chi_{\text{bar}0}$ ,  $\chi_{\text{bar}1}$ };
variables = {amult, abarmult,
umult, xmult, xbarmult};

```

---

There are  $7+4+5=16$  “physical parameters” here. The 7  $M_i$  are not “physical”. The result of this paper is to find constraints that reduce the number of “physical parameters” so that the tachyonic degrees of freedom are no longer present.

```

In[72]:= DimLessLagParams = Table[ki, {i, 1, 7}];
DimLessSourParams = Table[ei, {i, 1, 4}];
MassesForLag = Table[mi, {i, 1, 5}];
MassesForShifts = Table[Mi, {i, 1, 7}];

```

---

Sometimes it is useful to implement the following restrictions, rather than consider a large number of uninteresting cases with zeros for various masses or parameters.

```

In[75]:= ksnotzero := Thread[DimLessLagParams  $\neq$  0];
msnotzero := Thread[MassesForLag  $\neq$  0];

```

---

This notebook does not include any considerations relating to susy, and its ghosts:

```
In[77]:= cghosts = {c1, c0, cbar1, cbar0};
```

---

except that the form of the action does arise from the Susy nature of the E series of papers including the XM, and the ZX sector, as set out in E7.

Here are some lists made from the field variables

```
In[78]:= fermions =
  {ψ0, ψ1, ψbar0, ψbar1, λ0, λ1, λbar0, λbar1,
   χ0, χ1, χbar0, χbar1, φ0, φ1, φbar0, φbar1};
```

---

For each fermion we need a source, and we denote these by sour rather than source, since that is easier to pronounce and write.

```
In[79]:= sourfermions =
  {sourψ0, sourψ1, sourψbar0, sourψbar1,
   sourλ0, sourλ1, sourλbar0, sourλbar1,
   sourχ0, sourχ1, sourχbar0, sourχbar1,
   sourφ0, sourφ1, sourφbar0, sourφbar1};
```

---

The derivatives of the field variables, using the `pa` operators below, are an essential feature of this notebook. The D'Alembertian, `box`, is made from two derivatives `pa`. We need to convert it several

times to and from its  $pa$  form. The expressions  $propn$  are basically of the form  $1/(box + m^2)$  but often they are much more complicated than that, as will be seen. We use Mathematica's `Dot` function to keep track of the order in expressions. In fact we never evaluate the `Dot` product. It is used simply as a notation for a non-commutative product, and after the expressions are in canonical order, we will drop the `Dot`. But we will need the following in the meantime.

```
In[80]:= onepas = {pa{0,0}, pa{0,1}, pa{1,0}, pa{1,1}};
boxtopa = box → - pa{0,0} . pa{1,1} + pa{0,1} . pa{1,0} ;
commutepa = {pa{1,0} . pa{0,1} → pa{0,1} . pa{1,0} ,
  pa{0,1} . pa{0,0} → pa{0,0} . pa{0,1} ,
  pa{1,1} . pa{0,0} → pa{0,0} . pa{1,1} ,
  pa{1,1} . pa{1,0} → pa{1,0} . pa{1,1} , pa{1,1} . pa{0,1} ->
  pa{0,1} . pa{1,1} , pa{1,0} . pa{0,0} → pa{0,0} . pa{1,0} };
proptoright := (prop_) . (pa_) :=> (pa) . (prop) /;
  MemberQ[onepas, pa] && MemberQ[props, prop];
```

---

After we drop the `Dot`, it is useful to convert back to the  $box$  using:

```
In[81]:= patobox =
  {pa{0,0} → (1 / pa{1,1}) (-box + pa{0,1} pa{1,0}) ,
  pa{0,0}2 → (1 / pa{1,1})2 (-box + pa{0,1} pa{1,0})2};
```

We need 16 props here for the fermions. We include a factor 1 with the lambda field, to be consistent with papers E6 and E7.

```
In[82]:= props = {prop1, prop2, prop3, prop4, prop5,
  prop6, prop7, prop8, prop9, prop10, prop11,
  prop12, prop13, prop14, prop15, prop16};
```

This is where we will introduce the  $e_i$ . These are the source terms which can be used in the path integral form of the quantum field theory.

```
In[83]:= sourceterms :=
  e1 (sourphi0 . phi1 - sourphi1 . phi0 +
    sourphibar0 . phibar1 - sourphibar1 . phibar0 ) +
  e2 (sourchi0 . chi1 - sourchi1 . chi0 + sourchibar0 . chibar1 -
    sourchibar1 . chibar0 ) +
  e3 (sourlambda0 . lambda1 - sourlambda1 . lambda0 + sourlambdaibar0 . lambdaibar1 -
    sourlambdaibar1 . lambdaibar0 ) +
  e4 ( sourpsi0 . psi1 - sourpsi1 . psi0 +
    sourpsibar0 . psibar1 - sourpsibar1 . psibar0 );
```

Here are some replacement operators, which we will use to change expressions to a canonical form, so that we can add them together, and develop equations for the props:

```
In[84]:= DropZeroDots = { (aa_) . (0 cc_) . bb_ -> 0,
  (0 cc_) . bb_ -> 0 , (bb_) . (0) -> 0 } ; removeq =
```

```

Flatten[{Table[(aaa_).(bbb_ qn) → qn aaa.bbb,
  {n, 1, 8}], Table[(qn aaa_).(bbb_) →
  qn aaa.bbb, {n, 1, 8}]]];
minustoleft = {( -a_ ). b_ → - a.b,
  ( a_ ). ( - b_ ) → - a.b};
cbartoleft = {(y_).cbarx → cbarx.y } ;
ctoleft = {(y_).cx → cx.y } ;
canonicalc =
  {c1.c0 → c0.c1, cbar1.cbar0 → cbar0.cbar1};
removeinteger = { (aa_Integer ). bb_. cc_ →
  aa bb.cc, aa__ . ( bb_Integer cc_ ) →
  bb aa . cc, aa_Integer ( aab_Integer
  bb_ .cc_ ) . dd_ → aa aab bb.cc.dd } ;
removeminusone = { aa_ . (-1) → - aa , (-aa_ ).
  bb_ → - aa . bb, bb_ . (- cc_) → - bb .cc,
  bb_ . (- cc_).dd_ → - bb .cc .dd} ;
removerational =
  {aaa_ . ( bbb_Rational cc_ ) → bbb aaa . cc ,
  (bbb_Rational aaa_ ) . ( cc_ ) → bbb aaa . cc };
removeI = aa_ . ( I bb_ ) → I aa.bb;
removecomplex =
  { (aaa_ ). (bbb_Complex cc_ ) → bbb aaa.cc,
  (aaa_ bbb_Complex) . (cc_ ) → bbb aaa.cc};
valsofb = {b1 → 1, b2 → 1, b3 → 1,
  b4 → 1, b5 → -1, b6 → -1, b7 → 1,

```

```

b8 → -1, b9 → -1, b10 → 1, b11 → -1};
valsofq = {q1 → 1, q2 → 1, q3 → -1, q4 → 1,
q5 → 1, q6 → 1, q7 → 1, q8 → 1};
removedenom = {(pre_ / any_ ).post_ :=
(1 / any ) pre. post , pre_ . (post_ / any_ ) :=
(1 / any ) pre. post }; removedenom2 =
{ (pre_ / (any_ )2) . (post_ ) := pre.post / any2,
(pre_ ) . (post_ / (any_ )2) := pre.post / any2};

```

These are some more of the above:

```

In[88]:= removem = {Table[ ( mn aaa_ ).bbb_ → mn aaa.bbb,
{n, 1, 30}], Table[
( aaa_ ). (mn bbb_ ) → mn aaa.bbb, {n, 1, 30}],
Table[ ( Mn aaa_ ).bbb_ → Mn aaa.bbb,
{n, 1, 30}], Table[
( aaa_ ). (Mn bbb_ ) → Mn aaa.bbb, {n, 1, 30}]]];
removeb = { Table[ ( br aaa_ ).bbb_ → br aaa.bbb,
{r, 1, 11}], Table[
aaa_ . (br bbb_ ) → br aaa.bbb, {r, 1, 11}]]];
In[89]:= removemb = Flatten[{ removem, removeb}];

```



The following will implement putting the terms into a canonical order, and also this will implement integration by parts, which is always part of any Susy theory:

```
In[90]:= ordermixedterms :=
  factor_ fermi_ . anything_ . sour_ /;
  MemberQ[fermions, fermi] &&
  MemberQ[sourfermions, sour] =>
  - factor anything . sour . fermi ;
proponsouratleft :=
  (prop_ ) . (sour_ ) . (anything_ ) =>
  (sour) . (prop) . (anything) /; MemberQ[props,
  prop] && MemberQ[ sourfermions, sour];
paonsouratleft :=  (pa_ ) . (sour_ ) . (anything_ ) =>
  - (sour) . (pa) . (anything) /; ( MemberQ[onepas,
  pa] && MemberQ[ sourfermions, sour]);
```

Here are the pieces of the fermionic part of the free quadratic action, as discussed in the E papers. Susy is not really included here yet. If it is implemented simply, Susy would require some relations among these coefficients, for example  $k_1 = k_2$ . However we find that it is necessary, and indeed essential, to include counterterms that are discussed in E7, and these can also change the relations among the coefficients, as will be discussed in E9.

```
In[91]:= fermionsfromphibark1 =
  Total[Flatten[k1 Table[ (-1)(a+b)
    ϕMod[a+1,2] . box . pa{b,a} . ϕbarMod[b+1,2] ,
    {a, 0, 1}, {b, 0, 1} ] ] ];
```

```
In[92]:= fermionsfromchibark2 =
  Total[Flatten[k2 Table[
    (-1)(a+b) χMod[a+1,2] . pa{b,a} . χbarMod[b+1,2] ,
    {a, 0, 1}, {b, 0, 1} ] ] ];
```

```
fermionsfromphichimassm3 =
  { (ϕ0 . χ1 - ϕ1 . χ0 + ϕbar0 . χbar1 - ϕbar1 . χbar0) m32 };
```

```
In[93]:= fermionsfromphichik3 =
  ϕ0 . box . χ1 k3 - ϕ1 . box . χ0 k3 +
  ϕbar0 . box . χbar1 k3 - ϕbar1 . box . χbar0 k3;
```

```
In[94]:= fermionsfromlamlambark4 =
  Total[Flatten[ k4 Table[
    (-1)^(a+b) λMod[a+1,2] . pa{a,b} . λMod[b+1,2] ,
    {a, 0, 1}, {b, 0, 1} ]]] ;
```

There are no fermions in cL4 of E7. We also want the following complicated terms fermionsfrompsipsibarandmassesk5, with masses, These were discussed in E7.

```
In[95]:= fermionsfrompsipsibarandmassesk5 =
  { 1/2 k5 ( 2 ψ0 . pa{1,0} . ψ1 - 2 ψ0 . pa{1,1} . ψ0 -
    2 ψ1 . pa{0,0} . ψ1 + 2 ψ1 . pa{0,1} . ψ0 +
    i ψ0 . λ1 m1 - i ψ1 . λ0 m1 - i ψ0 . λ1 m1 +
    i ψ1 . λ0 m1 - 2 χ0 . ψ1 b11 m2 + 2 χ1 . ψ0 b11 m2 +
    b11 m2 - 2 χ0 . ψ1 b11 m2 + 2 χ1 . ψ0 b11 m2 +
    i φ0 . λ1 b4 m1 m2 - i φ1 . λ0 b4 m1 m2 -
    i φ0 . λ1 b4 m1 m2 + i φ1 . λ0 b4 m1 m2 -
    2 φ0 . pa{0,1} . φ1 m22 + 2 φ0 . pa{1,1} . φ0 m22 +
    2 φ1 . pa{0,0} . φ1 m22 - 2 φ1 . pa{1,0} . φ0 m22 ) } ;
```

We find it is essential to include counterterms. In E7 it was hoped and suggested that this might not be necessary. That hope was misguided, and the suggestion was wrong. They are essential, in fact.

In[96]:= **fermionsfromcounterterm**sk6k7 :=

$$\begin{aligned}
 & m_4 \left( \psi_0 \cdot pa_{\{1,1\}} \cdot \phi_0 + \psi_1 \cdot pa_{\{0,0\}} \cdot \phi_1 - \psi_0 \cdot pa_{\{1,0\}} \cdot \phi_1 \right. \\
 & \quad - \psi_1 \cdot pa_{\{0,1\}} \cdot \phi_0 + \psi_{\text{bar}0} \cdot pa_{\{1,1\}} \cdot \phi_{\text{bar}0} + \\
 & \quad \psi_{\text{bar}1} \cdot pa_{\{0,0\}} \cdot \phi_{\text{bar}1} - \psi_{\text{bar}1} \cdot pa_{\{1,0\}} \cdot \phi_{\text{bar}0} - \\
 & \quad \left. \psi_{\text{bar}0} \cdot pa_{\{0,1\}} \cdot \phi_{\text{bar}1} \right) + \\
 & k_6 \left( I \left( \lambda_0 \cdot pa_{\{1,1\}} \cdot \chi_0 + \lambda_1 \cdot pa_{\{0,0\}} \cdot \chi_1 - \right. \right. \\
 & \quad \left. \lambda_0 \cdot pa_{\{1,0\}} \cdot \chi_1 - \lambda_1 \cdot pa_{\{0,1\}} \cdot \chi_0 \right) \\
 & \quad - I \left( \lambda_{\text{bar}0} \cdot pa_{\{1,1\}} \cdot \chi_{\text{bar}0} + \right. \\
 & \quad \left. \lambda_{\text{bar}1} \cdot pa_{\{0,0\}} \cdot \chi_{\text{bar}1} - \lambda_{\text{bar}0} \cdot pa_{\{0,1\}} \cdot \chi_{\text{bar}1} - \right. \\
 & \quad \left. \lambda_{\text{bar}1} \cdot pa_{\{1,0\}} \cdot \chi_{\text{bar}0} \right) \left. \right) + \\
 & I k_7 \left( \lambda_0 \cdot \text{box} \cdot \phi_{\text{bar}1} - \lambda_1 \cdot \text{box} \cdot \phi_{\text{bar}0} - \lambda_{\text{bar}0} \cdot \text{box} \cdot \phi_1 \right. \\
 & \quad \left. + \lambda_{\text{bar}1} \cdot \text{box} \cdot \phi_0 \right) + I m_5^2 \\
 & \left( \lambda_0 \cdot \phi_{\text{bar}1} - \lambda_1 \cdot \phi_{\text{bar}0} - \lambda_{\text{bar}0} \cdot \phi_1 + \lambda_{\text{bar}1} \cdot \phi_0 \right);
 \end{aligned}$$

Here is the collection of the fermions for the quadratic action. We convert the boxes to partial derivatives, so that we do not have to include both kinds of derivatives, for the time being. Later we will convert the pa back to box, for certain purposes.

```
In[97]:= quadfermionlagrangian := Simplify[
  Total[Flatten[{fermionsfromphibark1 ,
    fermionsfromchibark2,
    fermionsfromphichimassm3,
    fermionsfromphichik3,
    fermionsfromlamlabark4,
    fermionsfrompsibarandmassesk5 ,
    fermionsfromcountertermk6k7 ,
    sourceterms}] /. boxtopa]]
```

```
In[98]:=
```

---

Now we consider calculation of the equations that determine the 16 functions  $\text{propn}$ . These require the following fermionic shifts, which arise from the form of the fermionic action above. In fact these are the most general shifts possible, given the properties of the fields, and that is probably crucial. There are 16  $\text{propn}$  which correspond to a shift of each of the four fermion fields to each of the other four fermion fields, and that is why we must include the counterterms referred to above. The sub-indices here are determined so that Lorentz invariance remains manifest.

$$\begin{aligned}
\text{In[99]:= } \psi\text{shift0} = & \psi_0 \rightarrow \psi_0 + \text{pa}_{\{0,0\}} \cdot \text{prop10} \cdot \text{sour}\psi\text{bar}_1 - \\
& \text{pa}_{\{0,1\}} \cdot \text{prop10} \cdot \text{sour}\psi\text{bar}_0 + \\
& \text{I M}_1 \text{ prop11} \cdot \text{sour}\lambda_0 + \text{M}_2 \text{ prop12} \cdot \text{sour}\chi\text{bar}_0 + \\
& \frac{1}{\text{M}_3} \text{pa}_{\{0,0\}} \cdot \text{prop13} \cdot \text{sour}\phi_1 - \\
& \frac{1}{\text{M}_3} \text{pa}_{\{0,1\}} \cdot \text{prop13} \cdot \text{sour}\phi_0 ;
\end{aligned}$$

$$\begin{aligned}
\psi\text{shift1} = & \psi_1 \rightarrow \psi_1 + \text{pa}_{\{1,0\}} \cdot \text{prop10} \cdot \text{sour}\psi\text{bar}_1 - \\
& \text{pa}_{\{1,1\}} \cdot \text{prop10} \cdot \text{sour}\psi\text{bar}_0 + \\
& \text{I M}_1 \text{ prop11} \cdot \text{sour}\lambda_1 + \text{M}_2 \text{ prop12} \cdot \text{sour}\chi\text{bar}_1 + \\
& \frac{1}{\text{M}_3} \text{pa}_{\{1,0\}} \cdot \text{prop13} \cdot \text{sour}\phi_1 - \\
& \frac{1}{\text{M}_3} \text{pa}_{\{1,1\}} \cdot \text{prop13} \cdot \text{sour}\phi_0 ; \psi\text{barshift0} =
\end{aligned}$$

$$\begin{aligned}
\psi\text{bar}_0 \rightarrow & \psi\text{bar}_0 + \text{pa}_{\{0,0\}} \cdot \text{prop10} \cdot \text{sour}\psi_1 - \text{pa}_{\{1,0\}} \cdot \\
& \text{prop10} \cdot \text{sour}\psi_0 - \text{I M}_1 \text{ prop11} \cdot \text{sour}\lambda\text{bar}_0 + \text{M}_2 \\
& \text{prop12} \cdot \text{sour}\chi_0 + \frac{1}{\text{M}_3} \text{pa}_{\{0,0\}} \cdot \text{prop13} \cdot \text{sour}\phi\text{bar}_1 - \\
& \frac{1}{\text{M}_3} \text{pa}_{\{1,0\}} \cdot \text{prop13} \cdot \text{sour}\phi\text{bar}_0 ; \psi\text{barshift1} =
\end{aligned}$$

$$\begin{aligned}
\psi\text{bar}_1 \rightarrow & \psi\text{bar}_1 + \text{pa}_{\{0,1\}} \cdot \text{prop10} \cdot \text{sour}\psi_1 - \text{pa}_{\{1,1\}} \cdot \\
& \text{prop10} \cdot \text{sour}\psi_0 - \text{I M}_1 \text{ prop11} \cdot \text{sour}\lambda\text{bar}_1 + \text{M}_2 \\
& \text{prop12} \cdot \text{sour}\chi_1 + \frac{1}{\text{M}_3} \text{pa}_{\{0,1\}} \cdot \text{prop13} \cdot \text{sour}\phi\text{bar}_1 - \\
& \frac{1}{\text{M}_3} \text{pa}_{\{1,1\}} \cdot \text{prop13} \cdot \text{sour}\phi\text{bar}_0 ;
\end{aligned}$$

```

In[100]:=  $\psi\text{shifts} =$ 
           {  $\psi\text{shift0}$ ,  $\psi\text{shift1}$ ,  $\psi\text{barshift0}$ ,  $\psi\text{barshift1}$  };

In[101]:=  $\lambda\text{shift0} =$ 
            $\lambda_0 \rightarrow \lambda_0 + \text{pa}_{\{0,0\}} \cdot \text{prop7} \cdot \text{sour}\lambda\text{bar}_1 -$ 
            $\text{pa}_{\{0,1\}} \cdot \text{prop7} \cdot \text{sour}\lambda\text{bar}_0 +$ 
            $\text{I } M_4 \text{ prop8} \cdot \text{sour}\psi_0 + \text{I prop9} \cdot \text{sour}\phi\text{bar}_0 +$ 
            $\text{I pa}_{\{0,0\}} \cdot \text{prop14} \cdot \text{sour}\chi_1 -$ 
            $\text{I pa}_{\{0,1\}} \cdot \text{prop14} \cdot \text{sour}\chi_0;$ 
 $\lambda\text{shift1} = \lambda_1 \rightarrow \lambda_1 + \text{pa}_{\{1,0\}} \cdot \text{prop7} \cdot \text{sour}\lambda\text{bar}_1 -$ 
            $\text{pa}_{\{1,1\}} \cdot \text{prop7} \cdot \text{sour}\lambda\text{bar}_0 + \text{I } M_4 \text{ prop8} \cdot \text{sour}\psi_1 +$ 
            $\text{I prop9} \cdot \text{sour}\phi\text{bar}_1 + \text{I pa}_{\{1,0\}} \cdot \text{prop14} \cdot \text{sour}\chi_1 -$ 
            $\text{I pa}_{\{1,1\}} \cdot \text{prop14} \cdot \text{sour}\chi_0;$ 
 $\lambda\text{barshift0} = \lambda\text{bar}_0 \rightarrow \lambda\text{bar}_0 +$ 
            $\text{pa}_{\{0,0\}} \cdot \text{prop7} \cdot \text{sour}\lambda_1 - \text{pa}_{\{1,0\}} \cdot \text{prop7} \cdot \text{sour}\lambda_0 -$ 
            $\text{I } M_4 \text{ prop8} \cdot \text{sour}\psi\text{bar}_0 - \text{I prop9} \cdot \text{sour}\phi_0 -$ 
            $\text{I pa}_{\{0,0\}} \cdot \text{prop14} \cdot \text{sour}\chi\text{bar}_1 +$ 
            $\text{I pa}_{\{1,0\}} \cdot \text{prop14} \cdot \text{sour}\chi\text{bar}_0;$ 
 $\lambda\text{barshift1} = \lambda\text{bar}_1 \rightarrow \lambda\text{bar}_1 +$ 
            $\text{pa}_{\{0,1\}} \cdot \text{prop7} \cdot \text{sour}\lambda_1 - \text{pa}_{\{1,1\}} \cdot \text{prop7} \cdot \text{sour}\lambda_0 -$ 
            $\text{I } M_4 \text{ prop8} \cdot \text{sour}\psi\text{bar}_1 - \text{I prop9} \cdot \text{sour}\phi_1 -$ 
            $\text{I pa}_{\{0,1\}} \cdot \text{prop14} \cdot \text{sour}\chi\text{bar}_1 +$ 
            $\text{I pa}_{\{1,1\}} \cdot \text{prop14} \cdot \text{sour}\chi\text{bar}_0;$ 

In[103]:=  $\lambda\text{shifts} =$ 
           {  $\lambda\text{shift0}$ ,  $\lambda\text{shift1}$ ,  $\lambda\text{barshift0}$ ,  $\lambda\text{barshift1}$  };

```



In[104]:=  $\chi\text{shift0} =$

$$\begin{aligned} \chi_0 \rightarrow & \chi_0 + \text{pa}_{\{0,0\}} \cdot \text{prop4} \cdot \text{sour}\chi\text{bar}_1 - \\ & \text{pa}_{\{1,0\}} \cdot \text{prop4} \cdot \text{sour}\chi\text{bar}_0 + \\ & \text{prop5} \cdot \text{sour}\phi_0 + M_5 \text{ prop6} \cdot \text{sour}\psi\text{bar}_0 + \\ & \text{I pa}_{\{0,0\}} \cdot \text{prop15} \cdot \text{sour}\lambda_1 - \\ & \text{I pa}_{\{1,0\}} \cdot \text{prop15} \cdot \text{sour}\lambda_0 ; \end{aligned}$$

$$\begin{aligned} \chi\text{shift1} = \chi_1 \rightarrow & \chi_1 + \text{pa}_{\{0,1\}} \cdot \text{prop4} \cdot \text{sour}\chi\text{bar}_1 - \\ & \text{pa}_{\{1,1\}} \cdot \text{prop4} \cdot \text{sour}\chi\text{bar}_0 + \\ & \text{prop5} \cdot \text{sour}\phi_1 + M_5 \text{ prop6} \cdot \text{sour}\psi\text{bar}_1 + \\ & \text{I pa}_{\{0,1\}} \cdot \text{prop15} \cdot \text{sour}\lambda_1 - \\ & \text{I pa}_{\{1,1\}} \cdot \text{prop15} \cdot \text{sour}\lambda_0 ; \end{aligned}$$

$$\begin{aligned} \chi\text{barshift0} = \chi\text{bar}_0 \rightarrow & \chi\text{bar}_0 + \\ & \text{pa}_{\{0,0\}} \cdot \text{prop4} \cdot \text{sour}\chi_1 - \text{pa}_{\{0,1\}} \cdot \text{prop4} \cdot \text{sour}\chi_0 + \\ & \text{prop5} \cdot \text{sour}\phi\text{bar}_0 + M_5 \text{ prop6} \cdot \text{sour}\psi_0 - \\ & \text{I pa}_{\{0,0\}} \cdot \text{prop15} \cdot \text{sour}\lambda\text{bar}_1 + \\ & \text{I pa}_{\{0,1\}} \cdot \text{prop15} \cdot \text{sour}\lambda\text{bar}_0 ; \end{aligned}$$

$$\begin{aligned} \chi\text{barshift1} = \chi\text{bar}_1 \rightarrow & \chi\text{bar}_1 + \\ & \text{pa}_{\{1,0\}} \cdot \text{prop4} \cdot \text{sour}\chi_1 - \text{pa}_{\{1,1\}} \cdot \text{prop4} \cdot \text{sour}\chi_0 + \\ & \text{prop5} \cdot \text{sour}\phi\text{bar}_1 + M_5 \text{ prop6} \cdot \text{sour}\psi_1 - \\ & \text{I pa}_{\{1,0\}} \cdot \text{prop15} \cdot \text{sour}\lambda\text{bar}_1 + \\ & \text{I pa}_{\{1,1\}} \cdot \text{prop15} \cdot \text{sour}\lambda\text{bar}_0 ; \end{aligned}$$

In[106]:=  $\chi\text{shifts} =$

$$\{\chi\text{shift0}, \chi\text{shift1}, \chi\text{barshift0}, \chi\text{barshift1}\};$$

In[107]:=  $\phi\text{shift0} =$

$$\begin{aligned}
\phi_\theta &\rightarrow \phi_\theta + (1/M_6^2) \text{pa}_{\{\theta,\theta\}} . \text{prop1.sour}\phi\text{bar}_1 - \\
&\quad (1/M_6^2) \text{pa}_{\{1,\theta\}} . \text{prop1.sour}\phi\text{bar}_\theta + \\
&\quad \text{prop2.sour}\chi_\theta + \text{I prop3 . sour}\lambda\text{bar}_\theta + \\
&\quad \frac{1}{M_7} \text{pa}_{\{\theta,\theta\}} . \text{prop16.sour}\psi_1 - \\
&\quad \frac{1}{M_7} \text{pa}_{\{1,\theta\}} . \text{prop16.sour}\psi_\theta ; \phi\text{shift1} = \\
\phi_1 &\rightarrow \phi_1 + (1/M_6^2) \text{pa}_{\{\theta,1\}} . \text{prop1.sour}\phi\text{bar}_1 - \\
&\quad (1/M_6^2) \text{pa}_{\{1,1\}} . \text{prop1.sour}\phi\text{bar}_\theta + \\
&\quad \text{prop2.sour}\chi_1 + \text{I prop3 . sour}\lambda\text{bar}_1 + \\
&\quad \frac{1}{M_7} \text{pa}_{\{\theta,1\}} . \text{prop16.sour}\psi_1 - \\
&\quad \frac{1}{M_7} \text{pa}_{\{1,1\}} . \text{prop16.sour}\psi_\theta ; \phi\text{barshift0} = \\
\phi\text{bar}_\theta &\rightarrow \phi\text{bar}_\theta + (1/M_6^2) \text{pa}_{\{\theta,\theta\}} . \text{prop1.sour}\phi_1 - \\
&\quad (1/M_6^2) \text{pa}_{\{\theta,1\}} . \text{prop1.sour}\phi_\theta + \\
&\quad \text{prop2.sour}\chi\text{bar}_\theta - \text{I prop3 . sour}\lambda_\theta + \\
&\quad \frac{1}{M_7} \text{pa}_{\{\theta,\theta\}} . \text{prop16.sour}\psi\text{bar}_1 - \\
&\quad \frac{1}{M_7} \text{pa}_{\{\theta,1\}} . \text{prop16.sour}\psi\text{bar}_\theta ; \phi\text{barshift1} = \\
\phi\text{bar}_1 &\rightarrow \phi\text{bar}_1 + (1/M_6^2) \text{pa}_{\{1,\theta\}} . \text{prop1.sour}\phi_1 - \\
&\quad (1/M_6^2) \text{pa}_{\{1,1\}} . \text{prop1.sour}\phi_\theta + \\
&\quad \text{prop2.sour}\chi\text{bar}_1 - \text{I prop3 . sour}\lambda_1 +
\end{aligned}$$

$$\frac{1}{M_7} \text{pa}_{\{1,0\}} \cdot \text{prop16.sour}\psi\text{bar}_1 -$$

$$\frac{1}{M_7} \text{pa}_{\{1,1\}} \cdot \text{prop16.sour}\psi\text{bar}_0;$$

```
In[108]:=  $\phi$ shifts =
           {  $\phi$ shift0,  $\phi$ shift1,  $\phi$ barshift0,  $\phi$ barshift1} ;
```

```
allshifts = Flatten[
           { $\phi$ shifts,  $\chi$ shifts,  $\lambda$ shifts,  $\psi$ shifts}];
```

```
In[110]:=
```

```
In[111]:= allshifts // Length
```

```
Out[111]= 16
```

**FERMION ACTION AND SHIFTS:** Now we start the derivation of the equations for the propn. The equations for propn come from requiring that the mixed terms that involve sourfermions and fermions all vanish. This ensures that in the path integral all we are left with is the generator of propagators. But we must calculate those terms by implementing the shifts and collecting terms, and then converting all terms to canonical forms. That requires quite a lot of manipulation, and the manipulation in this notebook is not really optimal here--it is more of an art than a science so far, and it certainly needs to be made more systematic. In fact these rules and their implementation come from examining the expressions, some of

them huge, to ensure that all necessary manipulations are included.

---

This is the Lagrangian

```
In[112]:= cLfermionstotalbig =
  Map[Distribute, Expand[ quadfermionlagrangian ],
    Infinity] //. removeminusone;
  cLfermionstotalbig // Length

Out[112]= 92
```

---

Here we shift the fields and reorganize the result a bit.

```
In[113]:= shiftedbig =
  Map[Distribute, cLfermionstotalbig /.
    allshifts, Infinity] /.
    removeminusone //. Flatten[
    removem] //. removedenom //.
    removedenom2 /. ordermixedterms /.
    DropZeroDots //. proptoright //.
    removeminusone //. commutepa //.
    removecomplex;
  shiftedbig // Length

Out[113]= 3360
```

```
In[114]:= shiftedbig;
```

---

Note that there are 3360 terms here. They can be viewed by removing the semicolon on the cell shiftedbig; We need to examine

them to make sure that the next steps work. Here we are putting the shifted Lagrangian into canonical form, so far as the mixed part goes

```
In[115]:= canonicalformmixedbig =
  Map[Distribute, shiftedbig, Infinity] //.
    removedenom //. removedenom2 //.
    removecomplex //.
    removeminusone //. proptoright //.
    commutepa //. removeminusone //.
    ordermixedterms //. proponsouratleft //.
    paonsouratleft //. removeminusone //.
    paonsouratleft //.
    removeminusone //.
    removedenom //.
    removedenom2;
canonicalformmixedbig // Length
```

```
Out[115]= 3248
```

This puts the above sum into a list

```
In[116]:= flatcanonbig =
  Flatten[canonicalformixedbig /. Plus -> List] /.
    paonsouratleft /.
      removeminusone /. paonsouratleft;
flatcanonbig // Length
```

```
Out[116]= 3248
```

Now we define a matrix of the 256 mixed terms with one source and one fermion:

```
In[117]:= tableanybig = Table[ Cases[flatcanonbig,
  aa_ Dot[sourfermions[[p]], any___,
    fermions[[q]] ]], {p, 1, 16}, {q, 1, 16}];
tableanybig // Dimensions
```

```
Out[117]= {16, 16}
```

```
In[118]:= TimeUsed[]
```

```
Out[118]= 6.501
```

This repeats the above in a different way:

```
In[119]:= tableofextractsbig :=
  Table[Extract[tableanybig, Position[
    tableanybig, aa_ sourfermions[[p]] .
      any___ . fermions[[q]] ] ], {p, 1, 16}
    , {q, 1, 16}]; tableofextractsbig //
  Dimensions
```

The following is zero:

```
In[160]:= tableofextractsbig - tableanybig;
In[120]:= TimeUsed[]
Out[120]= 6.673
```

This uses the above form, and removes the dot product for further use now:

```
In[121]:= tableofexpbig :=
  Table[ Cancel[ ( Total[tableofextractsbig[[p]][[
    q]]] /. Dot → Times ) /
    ( sourfermions[[p]] fermions[[q]] ) ],
    {p, 1, 16}, {q, 1, 16}] /. valsofb;
tableofexpbig // Dimensions
Out[121]= {16, 16}
```

---

Now we reduce that form to remove doubled terms

```
In[122]:= deldupsbig =
  DeleteDuplicates[Flatten[tableofexpbig]];
  deldupsbig // Length
```

```
Out[122]= 65
```

```
In[123]:= TimeUsed[]
```

```
Out[123]= 95.376
```

---

There are two kinds of terms in deldupsbig: terms with a derivative pa and terms without a derivative pa. First we single out the terms with a pa, and call them caspa:

```
In[124]:= caspa = Cases[Factor[deldupsbig], any_ pa_{p_, q_}];
  caspa // Length
```

```
Out[124]= 48
```

```
In[125]:=
```

---

These are the terms without any derivative which we call casnopa:

```
In[126]:= casnopa = Cases[Factor[deldupsbig],
  Except[any_ pa_{p_, q_}]]];
  casnopa // Length
```

```
Out[126]= 17
```



```
In[127]:= casnopaeqs = Thread[casnopa == 0];
          casnopaeqs // Length
```

```
Out[127]= 17
```

```
In[128]:= nopaset := Expand[Rest[casnopa] /. patobox];
          nopaset // Length
```

```
Out[128]= 16
```

```
In[129]:= nopaeqs = Thread[nopaset == 0];
          nopaeqs // Length
```

```
Out[129]= 16
```

Now we will examine the terms that do have a derivative. There are 4 kinds of derivative here with different indices, and we only need one of them:

```
In[130]:= expsfromcaspa00 =
          Cases[Factor[deldupsbig], any_ pa_{0,0} ] / pa_{0,0};
          expsfromcaspa00 // Length
```

```
Out[130]= 12
```

```
In[131]:= eqsfrompaterms = Thread[expsfromcaspa00 == 0];
          eqsfrompaterms // Length
```

```
Out[131]= 12
```

```
In[132]:= TimeUsed[]
```

```
Out[132]= 95.547
```

These two sets of equations above are easy to solve, and they

express props in terms of other props:

```
In[133]:= solsfromnopa = Flatten[Solve[nopaeqs, props]];
solsfromnopa // Length
```

... **Solve**: Equations may not give solutions for all "solve" variables.

Out[133]= 8

```
In[134]:= solsfrompa =
  Flatten[Solve[eqsfrompaterms, props]];
solsfrompa // Length
```

... **Solve**: Equations may not give solutions for all "solve" variables.

Out[134]= 8

```
In[135]:= simpsolsfromnopa =
  Simplify[solsfromnopa /. patobox];
In[136]:= simpsolsfrompa = Simplify[solsfrompa /. patobox];
```

---

We can collect all these relationships among props into one place:

```
In[137]:= simpallsols =
  Flatten[{simpsolsfromnopa /. Rule → Equal,
    simpsolsfrompa /. Rule → Equal}];
simpallsols // Length
```

Out[137]= 16

```
In[138]:= TimeUsed[]
```

```
Out[138]= 95.876
```

Now to further solve these equations for the props in terms of the parameters and the box, we define the four quartets. Each of these contains a closed set of equations for four props, and these are easy to solve for that set of four props. The author does not know why this happens, but presumably that question has an answer. The problem is that there are so many terms that it is a bit confusing.

```
In[139]:= firstquartet15913 = Together[
    Solve[{simpallsols[[1]], simpallsols[[5]],
           simpallsols[[11]], simpallsols[[15]] },
           {prop1, prop5, prop9, prop13}]];
```

```
In[140]:= secondquartet681016 = Together[
    Solve[{simpallsols[[8]], simpallsols[[2]],
           simpallsols[[10]], simpallsols[[12]] },
           {prop6, prop8, prop10, prop16}]];
```

```
In[141]:=
```

```
In[142]:= thirdquartet371115 = Together[
    Solve[{simpallsols[[3]], simpallsols[[7]],
           simpallsols[[13]], simpallsols[[16]] },
           {prop3, prop7, prop11, prop15}]];
```

```
In[143]:= fourthquartet241214 = Together[
    Solve[{simpallsols[[4]], simpallsols[[6]],
        simpallsols[[9]], simpallsols[[14]] },
    {prop2, prop4, prop12, prop14}]]];
```

---

Here is the set of all solutions for all 16 of the props. They are formidably long and complicated, and contain plenty of  $\text{box}^3$  and  $\text{box}^2$  terms, which mean that tachyons are present.

```
In[144]:= solsfrom4quartets = Flatten[
    {firstquartet15913, secondquartet681016,
    thirdquartet371115, fourthquartet241214}];
solsfrom4quartets;
```

---

A considerable amount of work (explained a bit in E8, but not shown in this notebook) was needed to find the following rules that map the complicated expressions to the normal form, without any obvious tachyons or higher derivatives in the propagators:

```
In[145]:= firstrule =  $\left\{ k_2 \rightarrow \frac{2 k_6 m_2}{m_1}, k_4 \rightarrow \frac{k_6 m_1}{2 m_2} \right\};$ 
```

In[146]:= **secondrule =**

$$\left\{ \begin{aligned} k_1 &\rightarrow \frac{k_3^2 m_1}{2 k_6 m_2} + \frac{2 k_6 m_2}{m_1} - \frac{2 k_3 m_3^2}{k_5 m_2^2} + \frac{2 k_6 m_3^4}{k_5^2 m_1 m_2^3}, \\ k_7 &\rightarrow \left( k_3 k_5 m_1^2 m_2 - 2 k_5 k_6 m_1 m_2^2 - \right. \\ &\quad \left. 2 k_6 m_1 m_3^2 + 4 k_6 m_2 m_5^2 \right) / \left( 2 k_5 m_1 m_2^2 \right), \\ m_4 &\rightarrow \left( k_5 m_1 m_2 \left( 2 k_7 m_3^2 + k_3 \left( k_5 m_1 m_2 - 2 m_5^2 \right) \right) \right) / \\ &\quad \left( 2 k_6 \left( k_5 m_1 m_2^2 + m_1 m_3^2 - 2 m_2 m_5^2 \right) \right) \end{aligned} \right\};$$

Applying these rules leads to a surprisingly simple form for the propn, as far as the presence of the D’Alembertian “box” goes. The are still complicated functions of the mass and dimensionless parameters however:

In[147]:= **newsols = Simplify[Flatten[solsfrom4quartets] /. firstrule /. secondrule];**

These can be viewed by removing the semicolon, as usual. We can express the mass pole in terms of the parameters as follows:

In[148]:= **mass = Solve[(2 box k<sub>6</sub> + k<sub>5</sub> m<sub>1</sub> m<sub>2</sub>) == 0, box]**

Out[148]=  $\left\{ \left\{ \text{box} \rightarrow -\frac{k_5 m_1 m_2}{2 k_6} \right\} \right\}$

In[149]:= **TimeUsed[]**

Out[149]= **100.203**

Here are some expressions converted to  $\text{\LaTeX}$ . Some of these are used in the paper E8:

```
In[150]:= quadfermionlagrangiannopa := Simplify[
      Total[Flatten[{fermionsfromphibark1 ,
        fermionsfromchichibark2,
        fermionsfromphichimassm3,
        fermionsfromphichik3,
        fermionsfromlam lambark4,
        fermionsfrompsipsibarandmassesk5 ,
        fermionsfromcountertermask6k7 ,
        sourceterms}] /. box → box]]

In[151]:= TeXForm[quadfermionlagrangiannopa];

In[152]:= TeXForm[firstrule];

In[153]:= TeXForm[secondrule];

In[154]:= TeXForm[ newsols];

In[155]:= TeXForm[{{box → -  $\frac{k_5 m_1 m_2}{2 k_6}$  }}];
```

```

In[156]:= TeXForm[Hold[ψshift0 =
      ψ0 → ψ0 + pa_{0,0} . prop10 . sourψbar1 -
      pa_{0,1} . prop10 . sourψbar0 +
      I M1 prop11 . sourλ0 + M2 prop12 . sourχbar0 +
      1/M3 pa_{0,0} . prop13 . sourφ1 -
      1/M3 pa_{0,1} . prop13 . sourφ0 ] ]];

In[157]:= TeXForm[Factor[Denominator[
      prop1 /. solsfrom4quartets] /. firstrule]]];

In[158]:= TimeUsed[]

Out[158]= 100.453

```
